# Supplementary material for: LEAGUE: Guided Skill Learning and Abstraction for Long-Horizon Manipulation
Source: arXiv:2210.12631 source file (2023-08-22)
Supplement: Supplementary file 1 [file appendix.tex]

\clearpage
\section{Appendix}
We provide the pseudo code of our proposed algorithm for skill learning and planning.

\begin{minipage}{0.48\linewidth}
\input{text/alg_plan}
\end{minipage}
\hfill
\begin{minipage}{0.48\linewidth}
\input{text/alg_learn}
\end{minipage}
